# Supplementary material for: Machine Learning in Precision Medicine to Preserve Privacy via Encryption
Source: arXiv:2102.03412 source file (2021-02-05)
Supplement: Supplementary file 1 [file SecAppendix.tex]

\section*{Appendix (Supplementary Material)}\label{sec:appendix}

\setcounter{section}{0}
\setcounter{page}{1}

\input{app-02.tex}

\input{app-05.tex}

\input{app-06.tex}

%%% Local Variables:
%%% mode: latex
%%% TeX-master: "main"
%%% End:
